# Supplementary material for: Continual Learning: Less Forgetting, More OOD Generalization via Adaptive Contrastive Replay
Source: arXiv:2410.07110 source file (2024-10-09)
Supplement: Supplementary file 1 [file 8_Supplementary.tex]

\begin{figure*}[t!]
  \centering
  \includegraphics[width=0.9\textwidth]{Styles/Image/Samples.png}
  \caption{Each column represents a CIFAR10 class. The first row contains 'simple' samples, the second row 'challenging' samples, and the third row 'hard' samples.}
  \label{fig:Samples}
\end{figure*}

\section{Experiments}

\paragraph{Hyperparameters.}
